# Supplementary material for: Natural orbitals and two-particle correlators as tools for analysis of effective exchange couplings in solids
Source: arXiv:2305.00325 source file (2023-04-29)
Supplement: Supplementary file 1 [file SI.pdf]

# Natural orbitals and two-particle correlators as tools for analysis of effective exchange couplings in solids

Pavel Pokhilko<sup>1</sup> and Dominika Zgid<sup>1,2</sup>

<sup>1</sup>*Department of Chemistry, University of Michigan, Ann Arbor, Michigan 48109, USA*

<sup>2</sup>*Department of Physics, University of Michigan, Ann Arbor, Michigan 48109, USA*

## 1. NiO

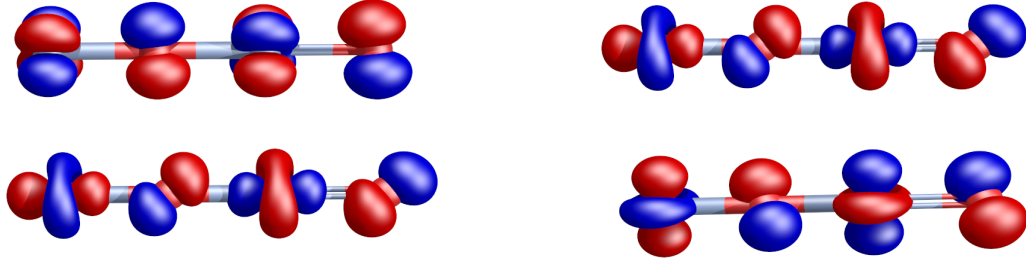

FIG. S1: Partly depopulated SA-NOs for broken-spin solutions at the  $\Gamma$  point of the NiO **cell 2** within GW, translated to different axes going through the nearest Ni–O bonds (SA-NOs for each axis are shown in columns).

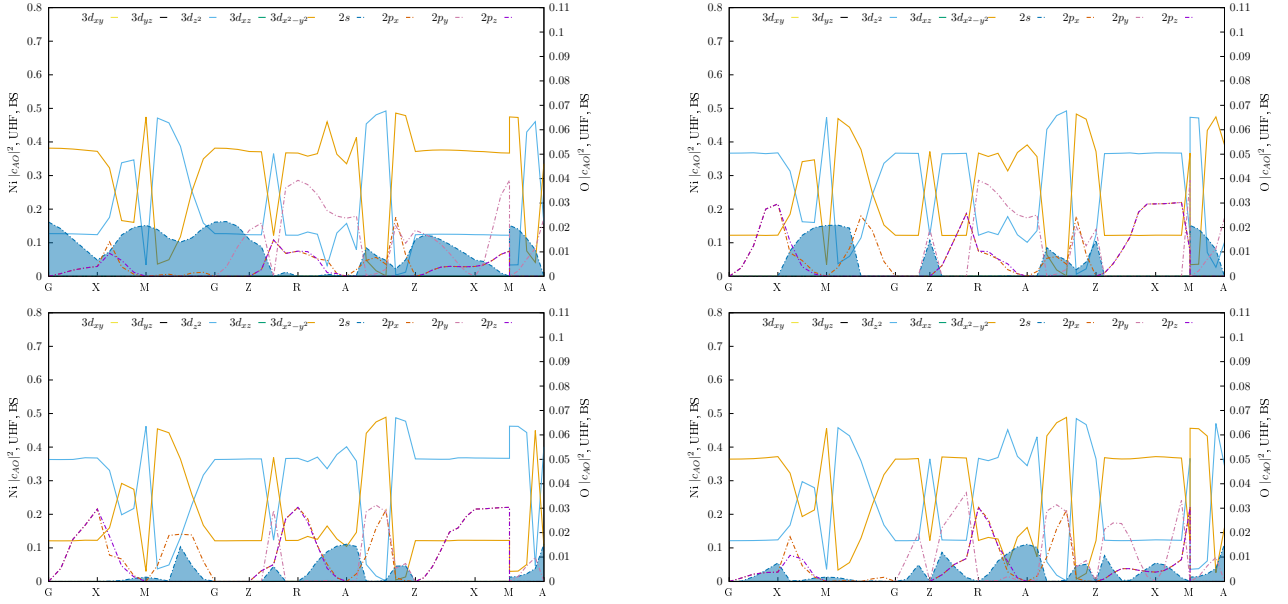

FIG. S2: Squared absolute values of atomic contributions to the UHF frontier SA-NOs along Wannier interpolation path in **cell 1**. The contributions of 3d AOs from the first nickel atom in the cell are shown by solid curves; the contributions of 2s and 2p AOs from the first oxygen atom are shown in dashed-dotted lines. The areas below 2s curves are filled to highlight contributions from the s-orbitals.

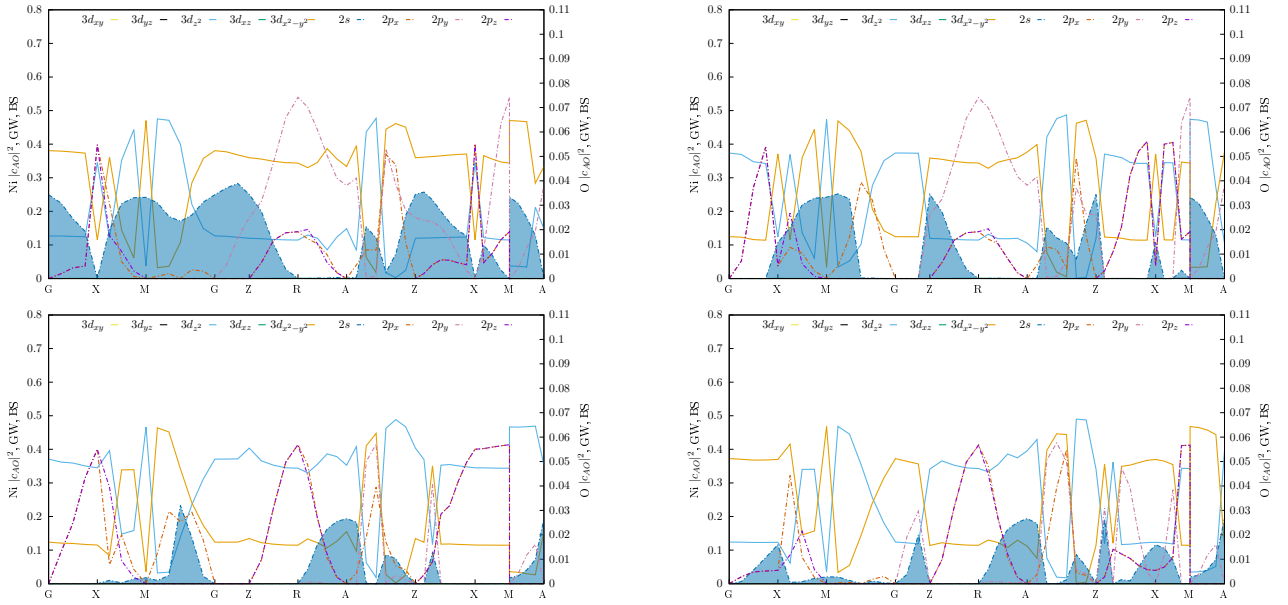

FIG. S3: Squared absolute values of atomic contributions to the GW frontier SA-NOs along Wannier interpolation path in **cell 1**. The contributions of 3d AOs from the first nickel atom in the cell are shown by solid curves; the contributions of 2s and 2p AOs from the first oxygen atom are shown in dashed-dotted lines. The areas below 2s curves are filled to highlight contributions from the s-orbitals.

## 2. CoO

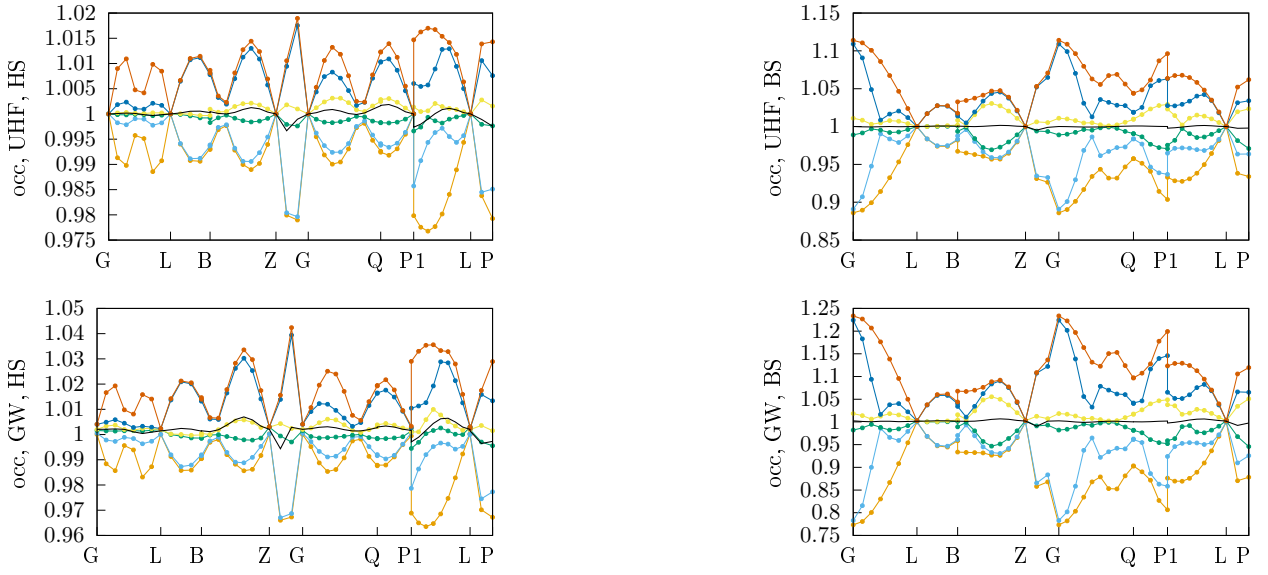

FIG. S4: Occupation numbers of the frontier SA-NOs for the k-points along the interpolated path for CoO in **cell 2** evaluated with UHF (top) and GW (down) with  $4 \times 4 \times 4$  grid for HS (left) and BS (right) solutions. The solid black line is the average of the occupancies of all 6 frontier SA-NOs at each k-point.

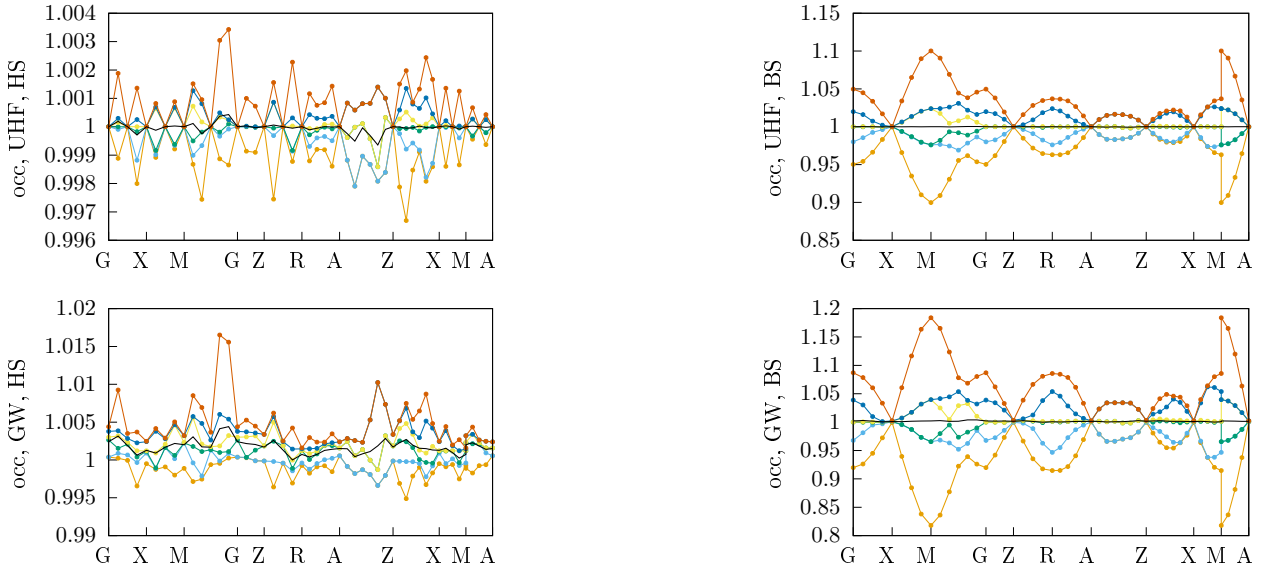

FIG. S5: Occupation numbers of the frontier SA-NOs for the k-points along the interpolated path for CoO in **cell 1** evaluated with UHF (top) and GW (down) with  $4 \times 4 \times 4$  grid for HS (left) and BS (right) solutions. The solid black line is the average of the occupancies of all 6 frontier SA-NOs at each k-point.

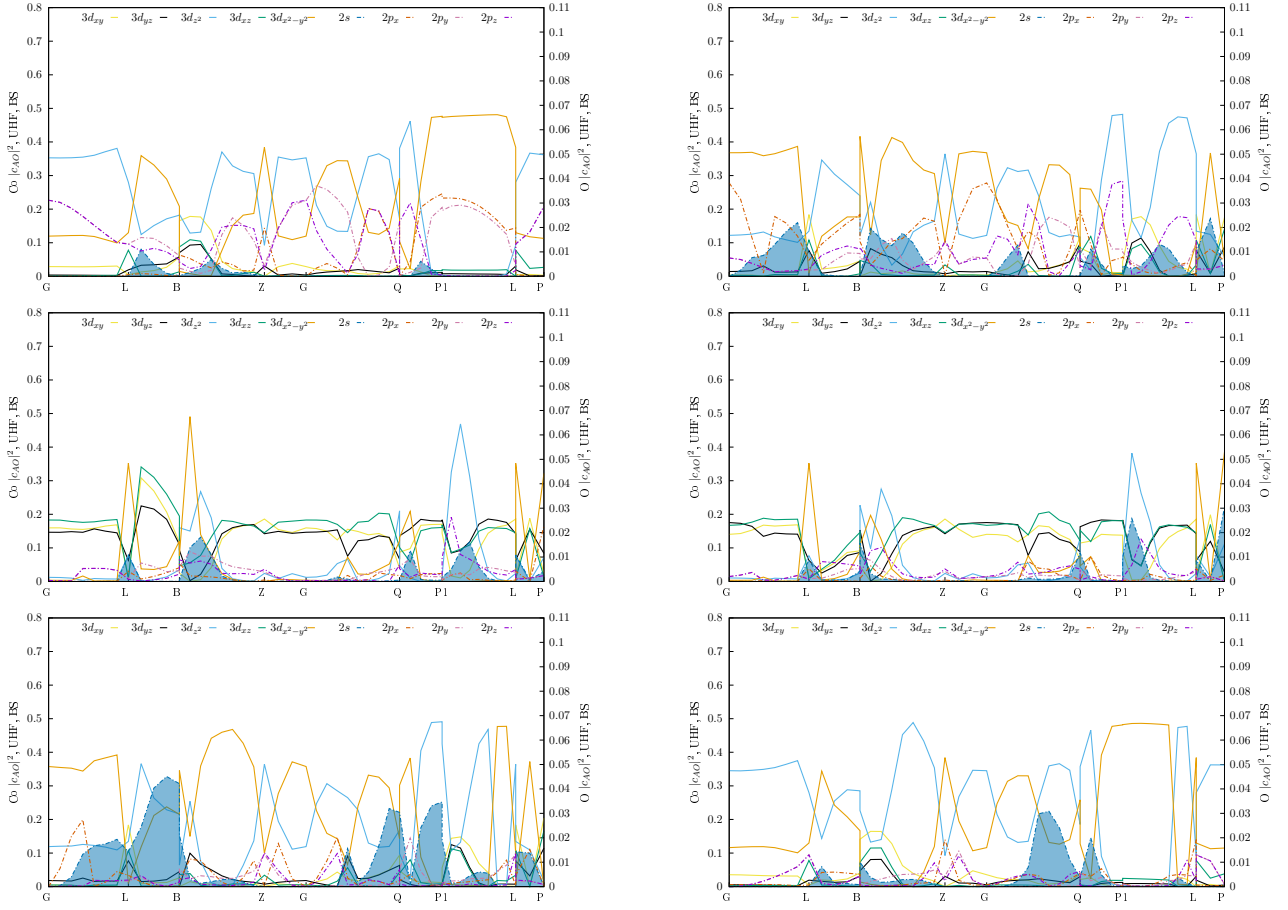

FIG. S6: Squared absolute values of atomic contributions to the UHF frontier SA-NOs along Wannier interpolation path in **cell 2** of CoO. The contributions of 3d AOs from the first Co atom in the cell are shown by solid curves; the contributions of 2s and 2p AOs from the first oxygen atom are shown in dashed-dotted lines. The areas below 2s curves are filled to highlight contributions from the s-orbitals.

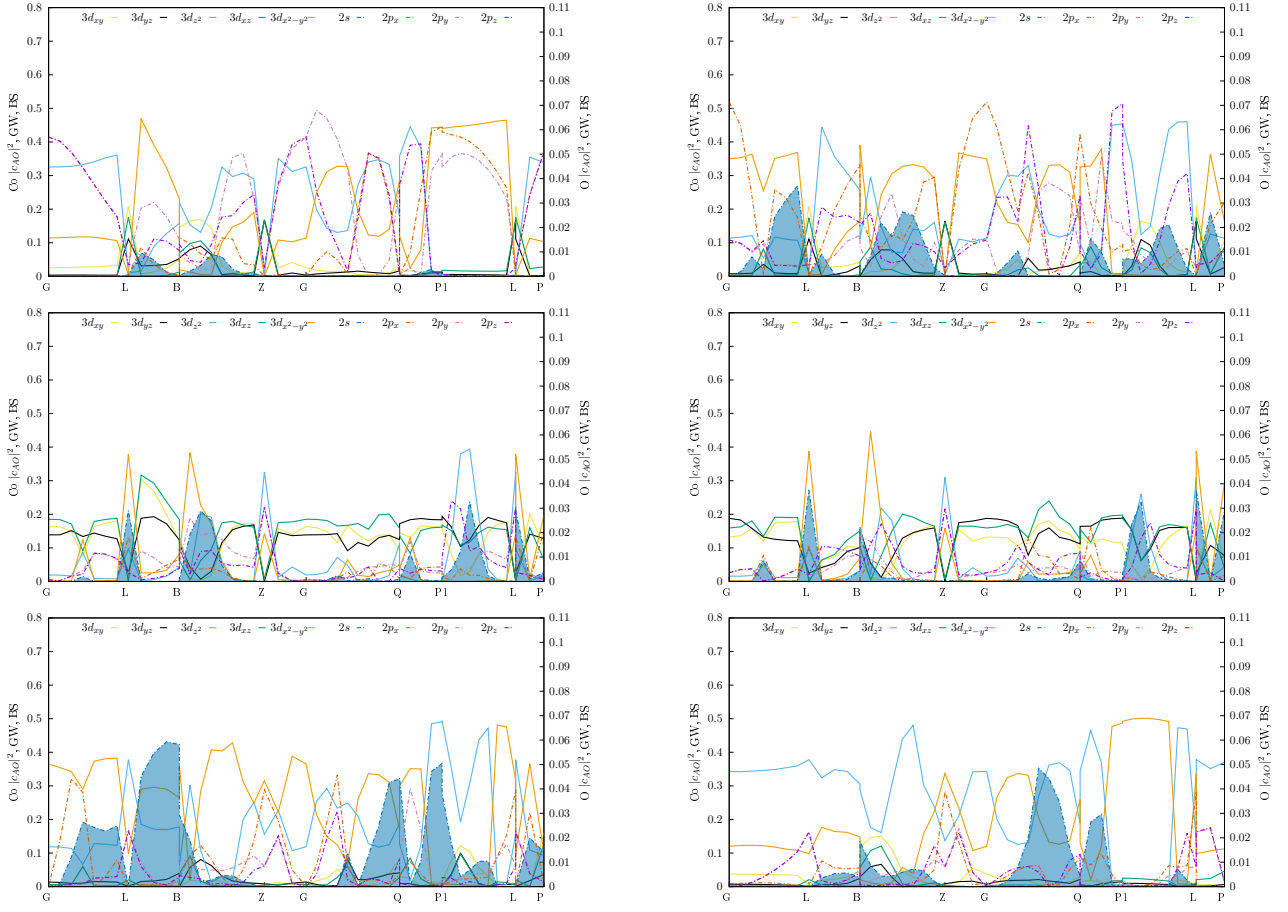

FIG. S7: Squared absolute values of atomic contributions to the GW frontier SA-NOs along Wannier interpolation path in **cell 2** of CoO. The contributions of 3d AOs from the first Co atom in the cell are shown by solid curves; the contributions of 2s and 2p AOs from the first oxygen atom are shown in dashed-dotted lines. The areas below 2s curves are filled to highlight contributions from the s-orbitals.

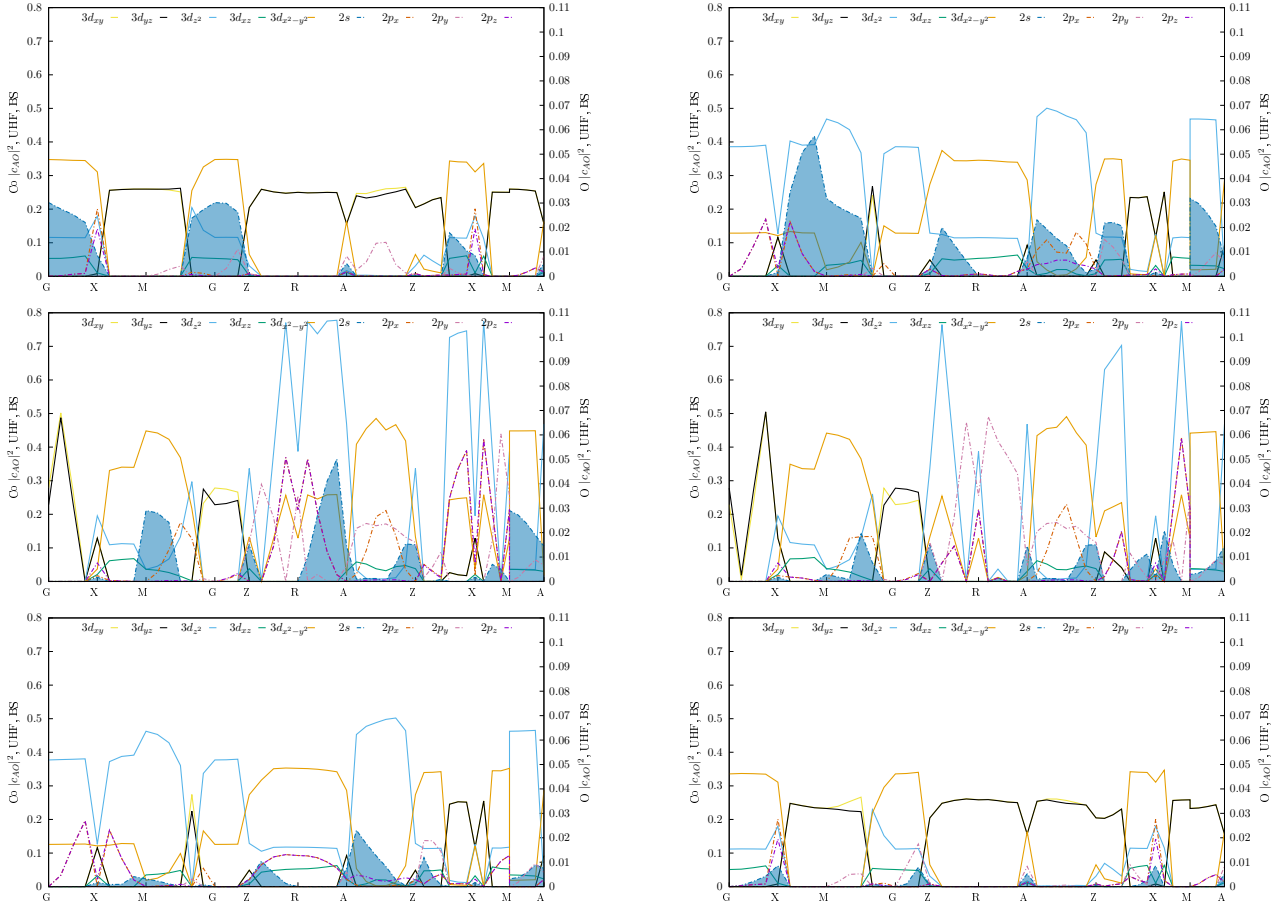

FIG. S8: Squared absolute values of atomic contributions to the UHF frontier SA-NOs along Wannier interpolation path in **cell 1** of CoO. The contributions of 3d AOs from the first Co atom in the cell are shown by solid curves; the contributions of 2s and 2p AOs from the first oxygen atom are shown in dashed-dotted lines. The areas below 2s curves are filled to highlight contributions from the s-orbitals.

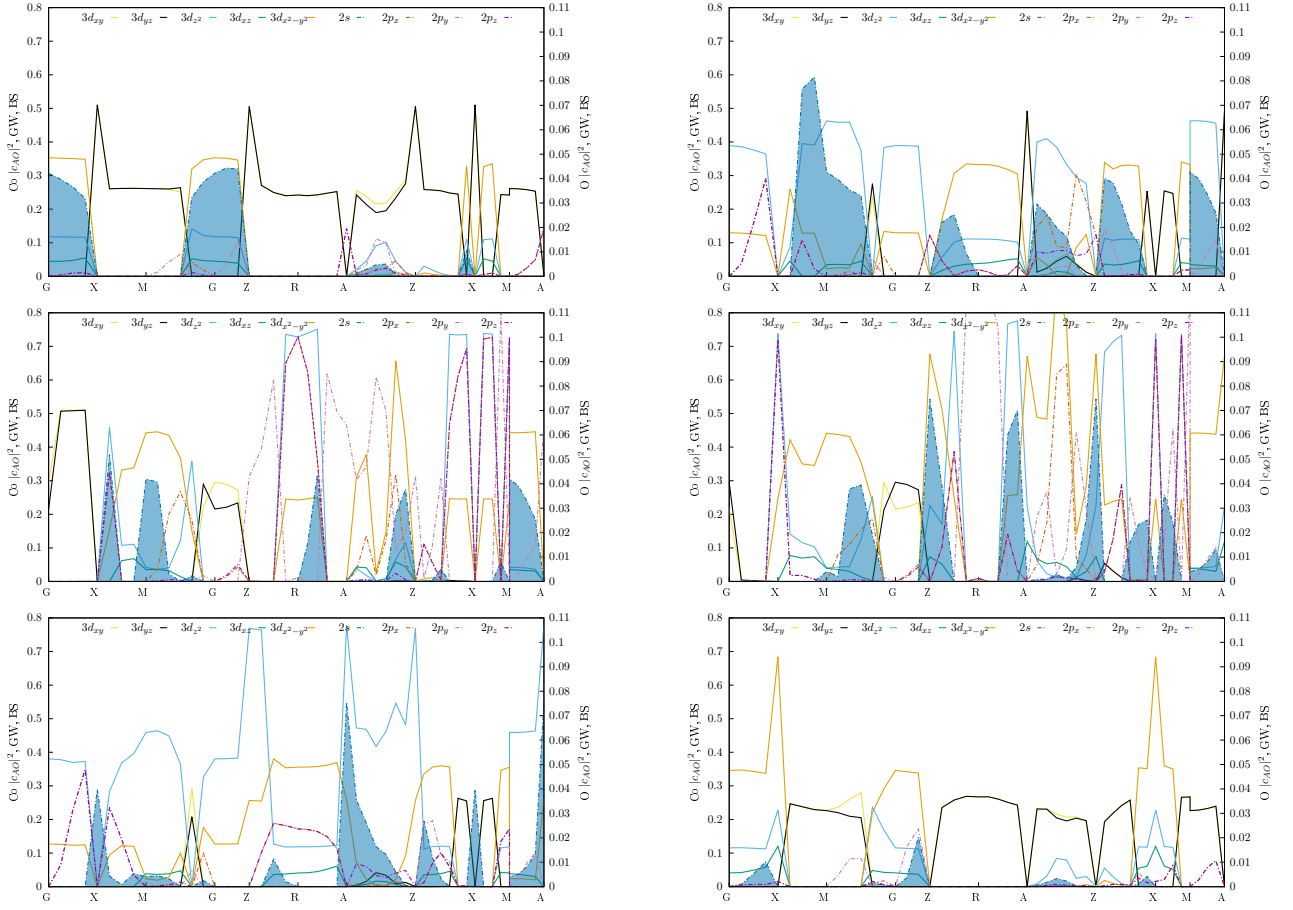

FIG. S9: Squared absolute values of atomic contributions to the GW frontier SA-NOs along Wannier interpolation path in **cell 1** of CoO. The contributions of 3d AOs from the first Co atom in the cell are shown by solid curves; the contributions of 2s and 2p AOs from the first oxygen atom are shown in dashed-dotted lines. The areas below 2s curves are filled to highlight contributions from the s-orbitals.

### 3. FeO

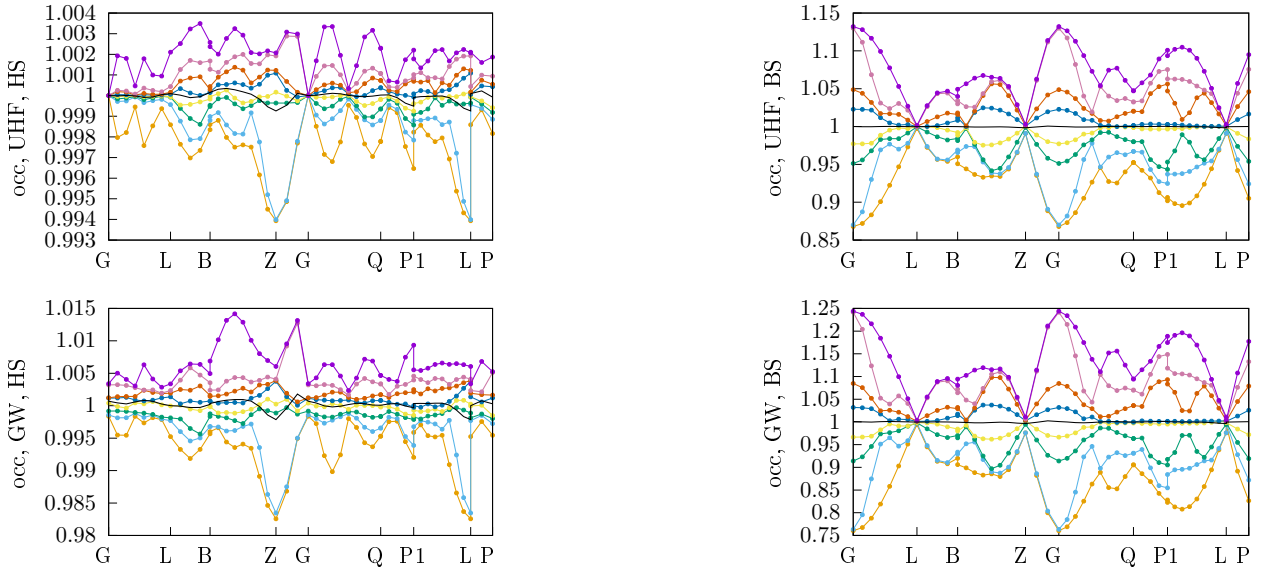

FIG. S10: Occupation numbers of the frontier SA-NOs for the k-points along the interpolated path for FeO in **cell 2** evaluated with UHF (top) and GW (down) with  $5 \times 5 \times 5$  grid for HS (left) and BS (right) solutions. The solid black line is the average of the occupancies of all 8 frontier SA-NOs at each k-point.

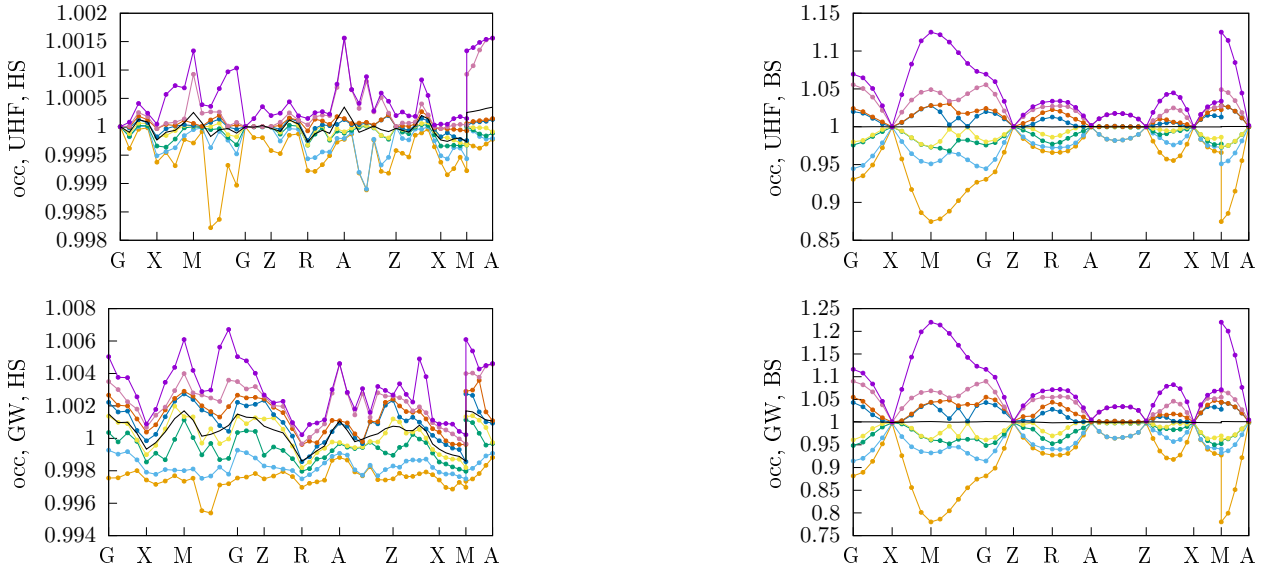

FIG. S11: Occupation numbers of the frontier SA-NOs for the k-points along the interpolated path for FeO in **cell 1** evaluated with UHF (top) and GW (down) with  $5 \times 5 \times 5$  grid for HS (left) and BS (right) solutions. The solid black line is the average of the occupancies of all 8 frontier SA-NOs at each k-point.



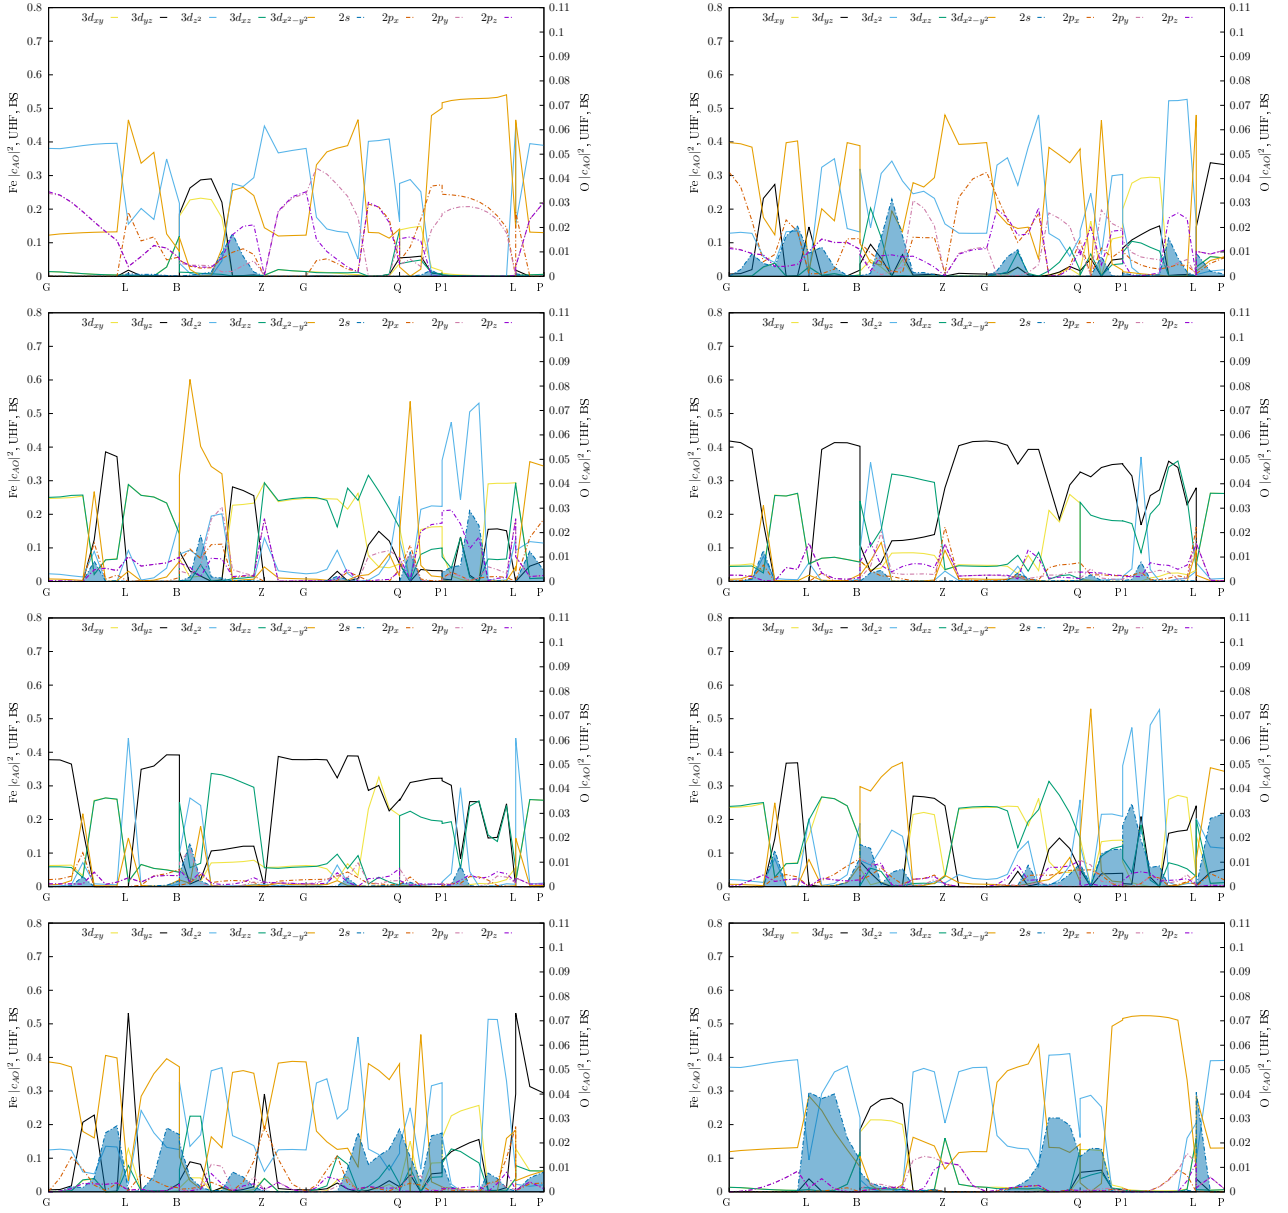

FIG. S12: Squared absolute values of atomic contributions to the UHF frontier SA-NOs along Wannier interpolation path in cell **2** of FeO. The contributions of 3d AOs from the first Fe atom in the cell are shown by solid curves; the contributions of 2s and 2p AOs from the first oxygen atom are shown in dashed-dotted lines. The areas below 2s curves are filled to highlight contributions from the s-orbitals.

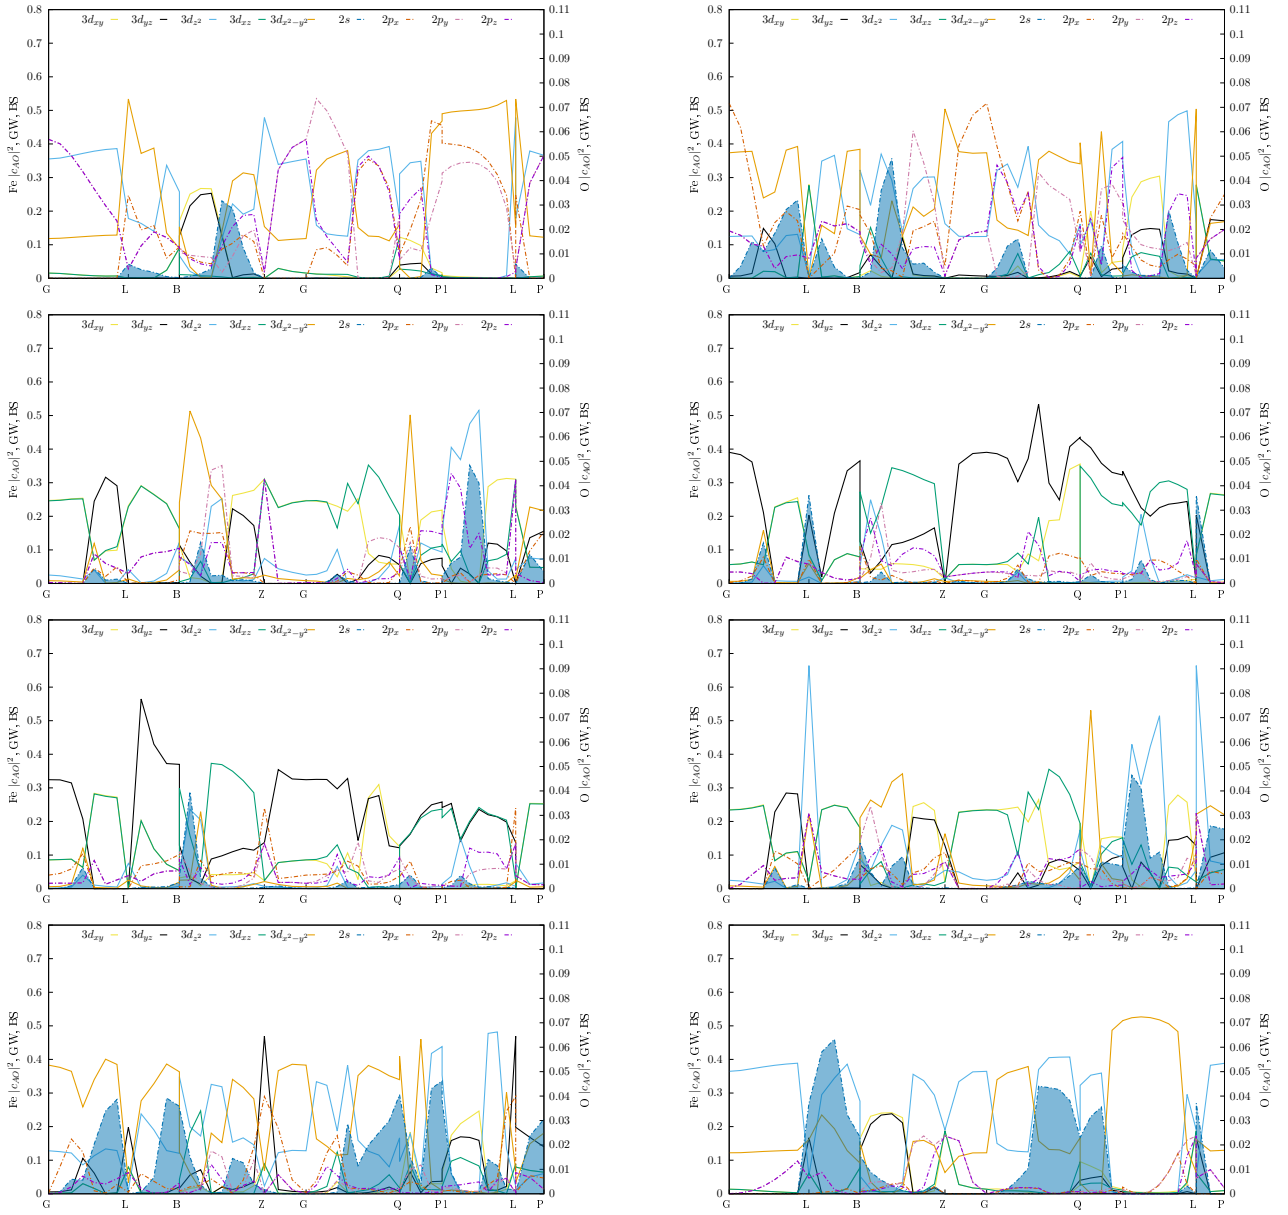

FIG. S13: Squared absolute values of atomic contributions to the GW frontier SA-NOs along Wannier interpolation path in cell **2** of FeO. The contributions of 3d AOs from the first Fe atom in the cell are shown by solid curves; the contributions of 2s and 2p AOs from the first oxygen atom are shown in dashed-dotted lines. The areas below 2s curves are filled to highlight contributions from the s-orbitals.

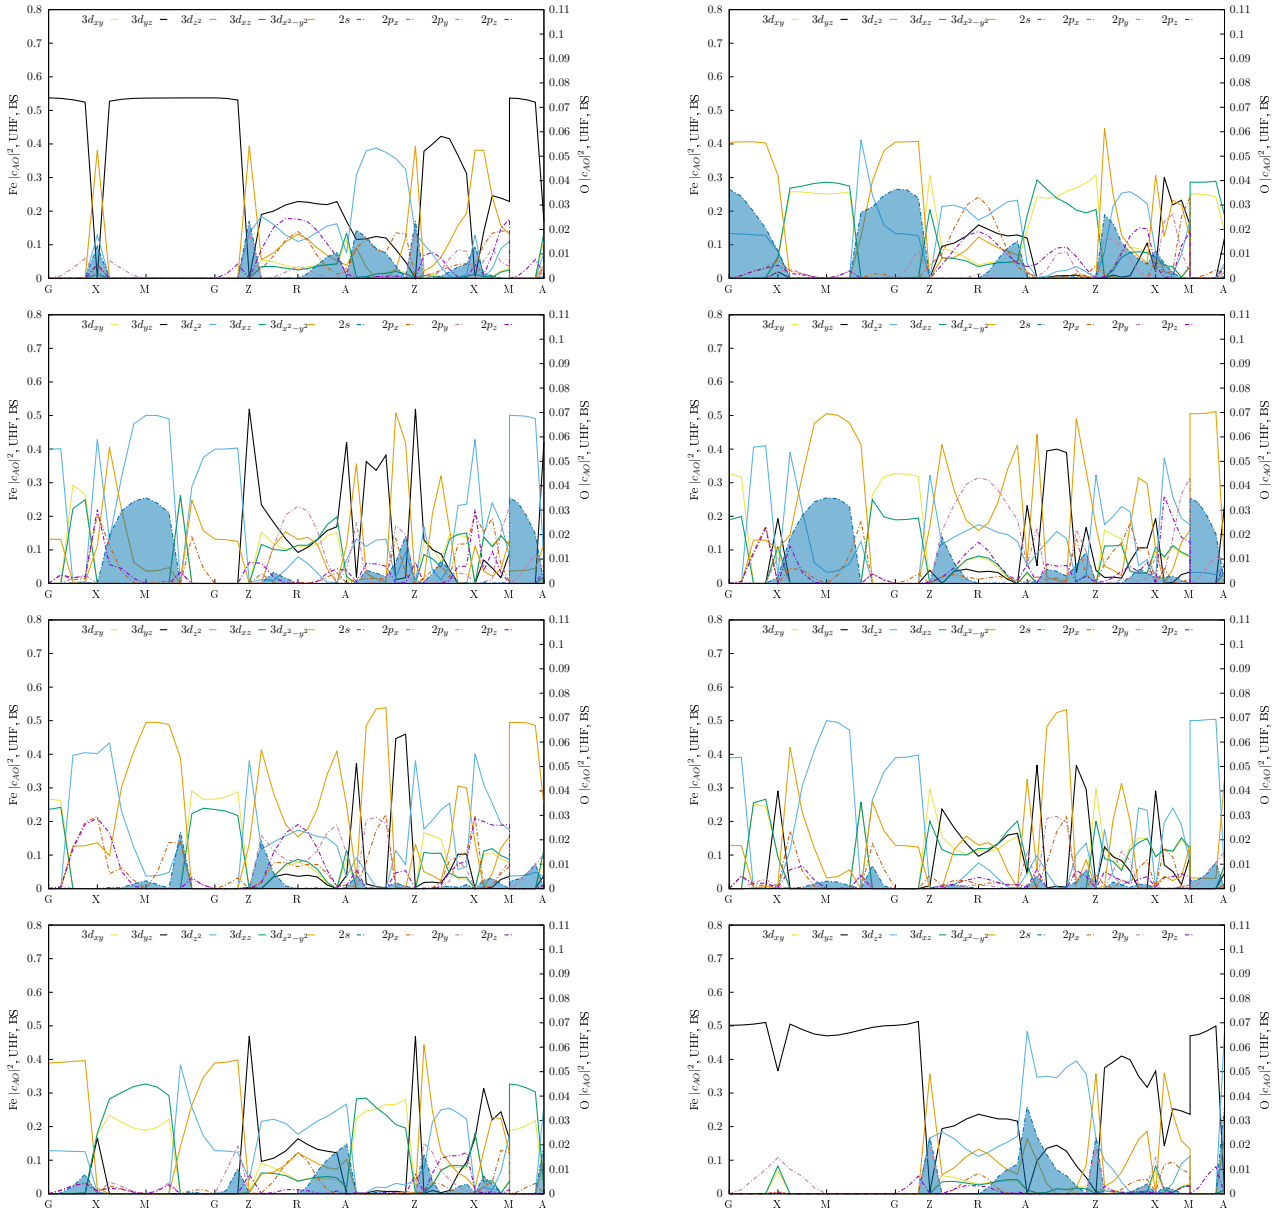

FIG. S14: Squared absolute values of atomic contributions to the UHF frontier SA-NOs along Wannier interpolation path in cell 1 of FeO. The contributions of  $3d$  AOs from the first Fe atom in the cell are shown by solid curves; the contributions of  $2s$  and  $2p$  AOs from the first oxygen atom are shown in dashed-dotted lines. The areas below  $2s$  curves are filled to highlight contributions from the  $s$ -orbitals.

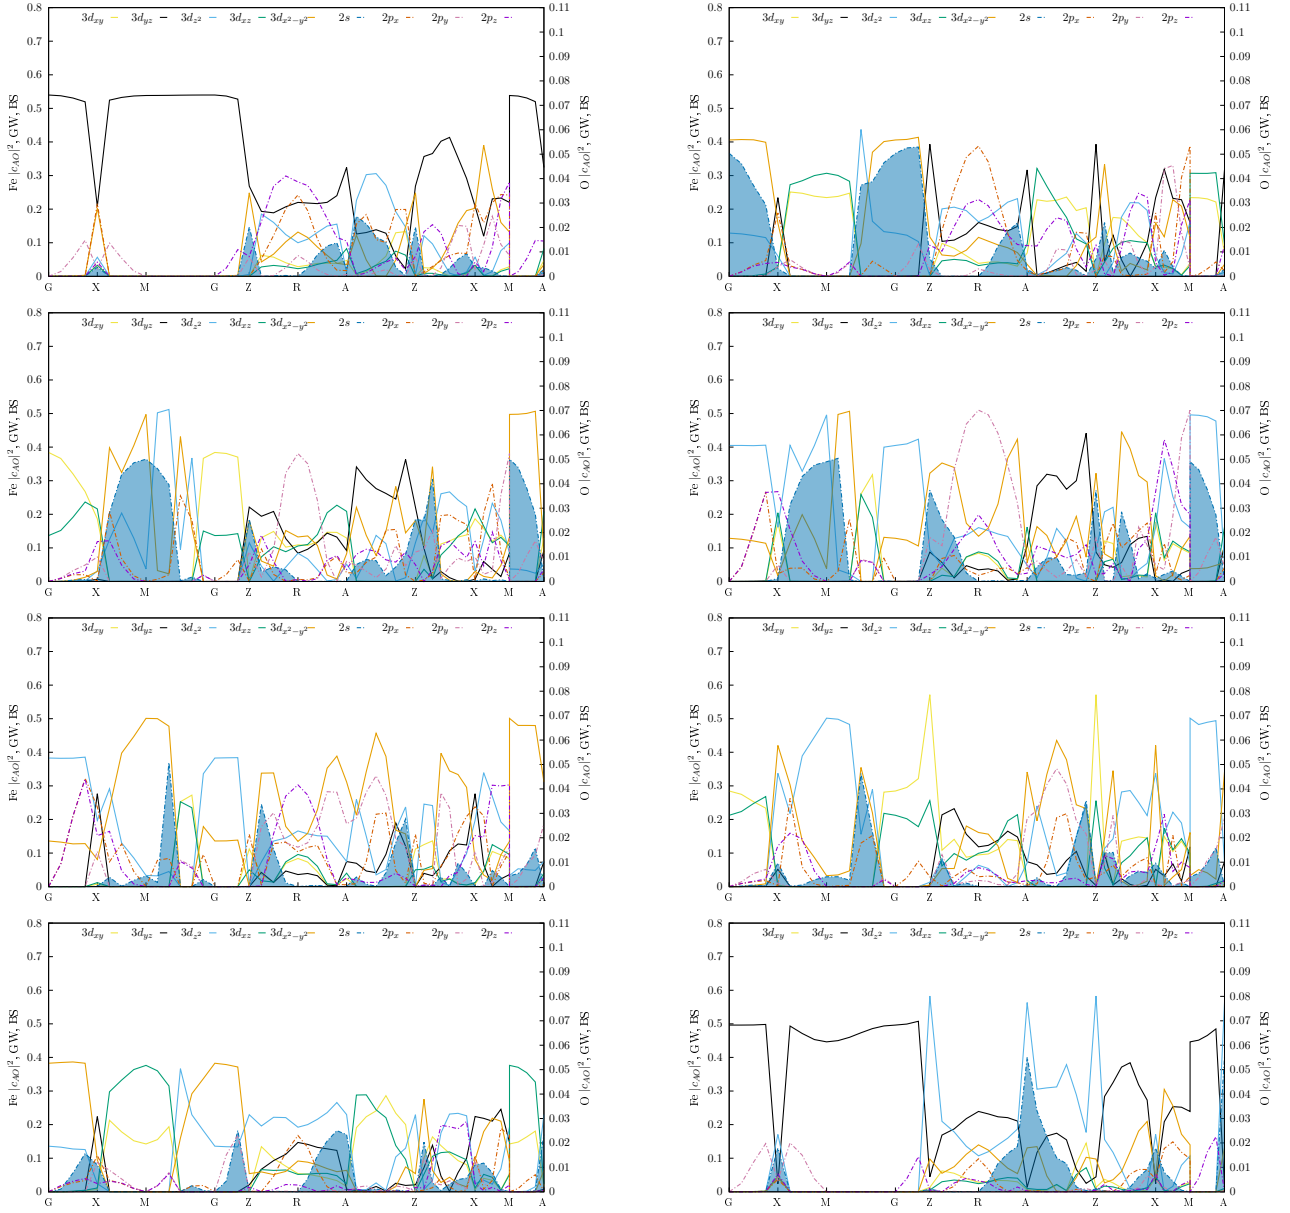

FIG. S15: Squared absolute values of atomic contributions to the GW frontier SA-NOs along Wannier interpolation path in cell 1 of FeO. The contributions of  $3d$  AOs from the first Fe atom in the cell are shown by solid curves; the contributions of  $2s$  and  $2p$  AOs from the first oxygen atom are shown in dashed-dotted lines. The areas below  $2s$  curves are filled to highlight contributions from the  $s$ -orbitals.
